# Supplementary material for: Low-energy phonons in Bi$_2$Sr$_2$CaCu$_2$O$_{8+\delta}$ and their possible interaction with electrons measured by inelastic neutron scattering
Source: arXiv:1702.04331 source file (2019-10-03)
Supplement: Supplementary file 1 [file Supplement.pdf]

# Low Energy Phonons in BSCCO and their Possible Interaction with Electrons Measured by Inelastic Neutron Scattering

A. Merritt, J.-P. Castellan, S. R. Park, J. A. Fernandez-Baca, G. D. Gu, D. Reznik

## Supplementary Material

During the course of the experiment many scans were taken, not all of which are shown in the main paper. We show some of the most important additional scans here, to supplement figures in the paper or to show a feature that is otherwise unexplained. Since the main thrust of paper is the change in the phonon eigenvector from  $h=0.15$  to  $h=0.25$ , the first two figures aid this point.

Fig. S1 shows the same momentum-energy cuts as Fig. 2 in the paper at final neutron energy 14.7 meV instead of 8 meV. This allows us to use the region near 10 meV, and also better shows some phonon dispersions in the zone. The phonon at 7 meV is seen more clearly and it is clear that there is no phonon in the 10 meV region that would have been missed in the other scans. Since scans at a final neutron energy of 8 meV have a higher energy resolution, those scans are reported in the main paper, but functionally they are the same. Scans at a different final energy also make it easier to identify spurious features, which we black out.

Fig. S2 shows longitudinal and transverse scans from the (2, 2, 0) Bragg peak. These scans were done at HFIR using a different, smaller BSCCO sample, but it still matches our data taken at LLB. In particular, the acoustic phonon that is very strong near the zone center (top left, S2a) undergoes a large reduction in intensity near  $q=0.3$  (top right, S2a) in the transverse mode. This momentum transfer directly coincides in both magnitude and direction with the suspected momentum transfer to explain the 10 meV kink in BSCCO, and shows that our conclusions drawn from our data are directly applicable. The same effect to a lesser degree is shown in S2b for the longitudinal mode.

Fig. S3 shows scans at several temperatures across H taken at an energy transfer of 1.5 meV. In particular, these scans were done to look for a peak near  $h=0.1$  to  $h=0.3$ . Such a peak might indicate very low-energy tails of the broad phonons. However, no significant signal in this scan was observed (the large increase for low H is from the Bragg peak). Thus, we can reasonably conclude that phonon lineshapes half-way to the zone boundary do not extend to this low energy.

Fig. S4 shows momentum-energy cuts along L near (0, 0, 14) and (0, 0, 12). These complement the momentum-energy cut Fig. 2c, and the peak positions reported in Fig. 2f, in the main paper.

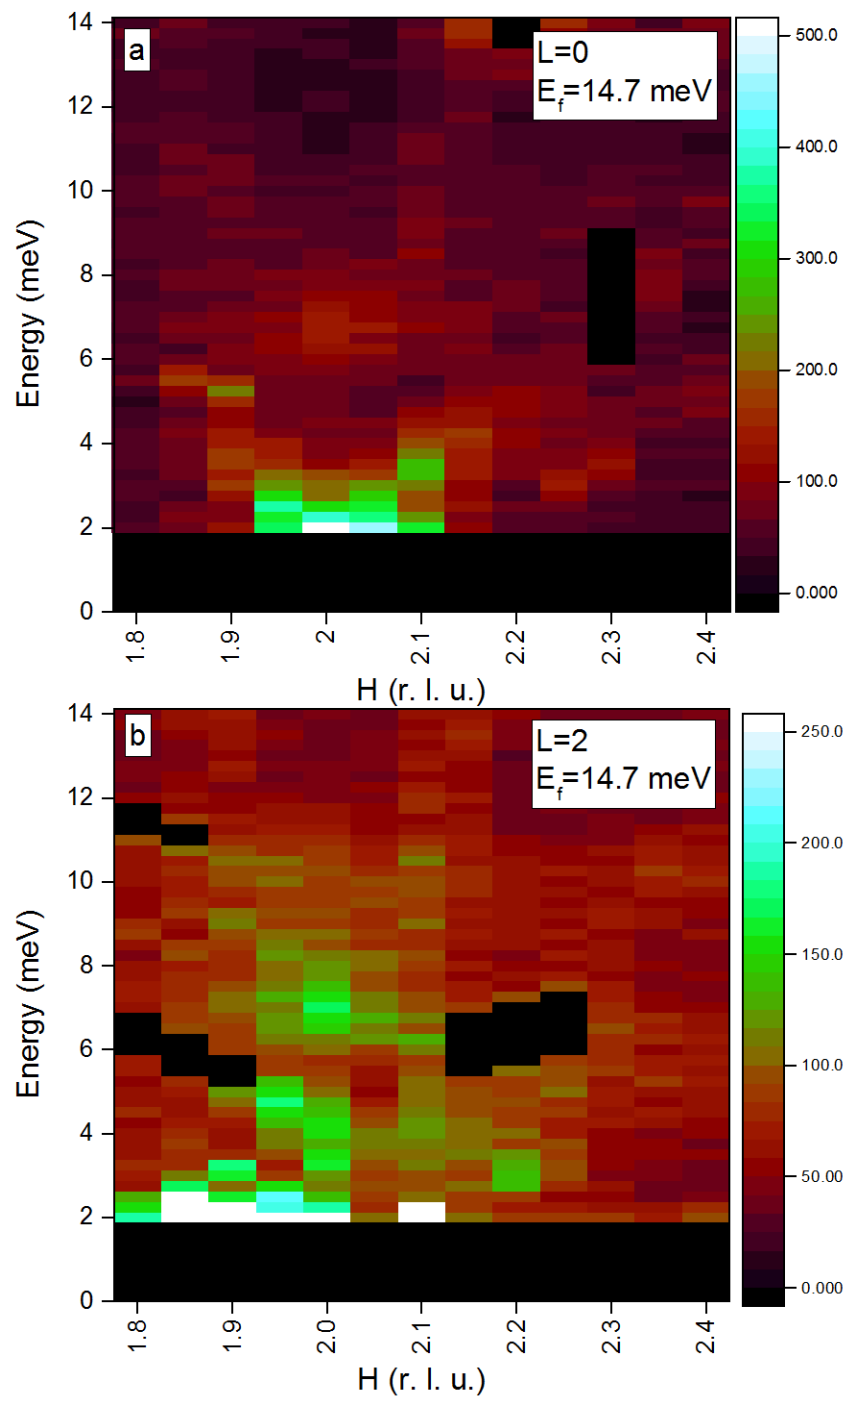

S1: Momentum-energy cuts for  $L=0$  (a) and  $L=2$  (b) at a final neutron energy of 14.7 meV and  $T = 10$  K.

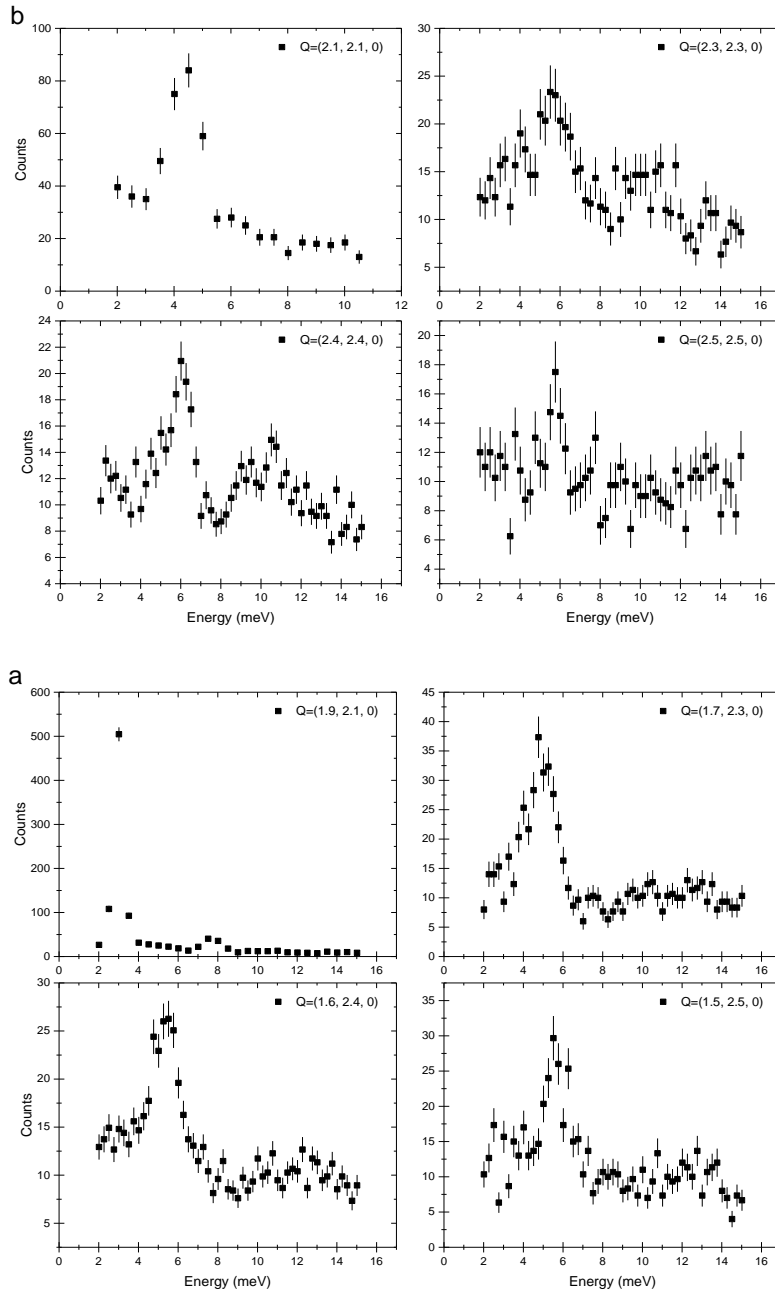

S2: Scans transverse (a) and longitudinal (b) from the (2, 2, 0) Bragg peak. Final neutron energy of 13.2 meV at  $T = 300$  K. Done at HFIR on different sample.

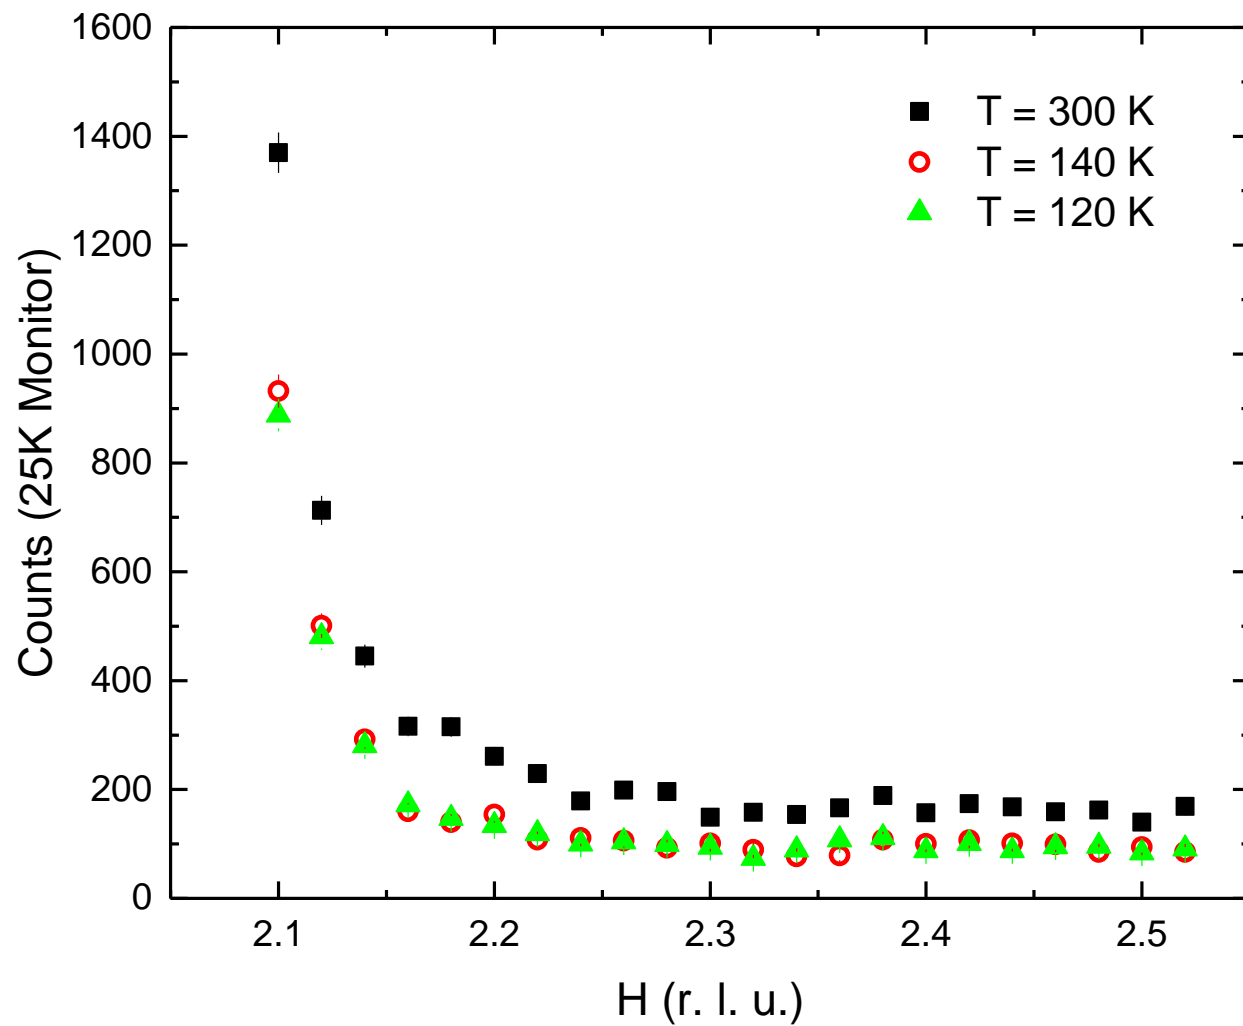

S3: Energy scans at  $L=0$ ,  $E_f = 13.2$  meV, several temperatures. Note the lack of any signal indicating a tail at low energy across the scan range.

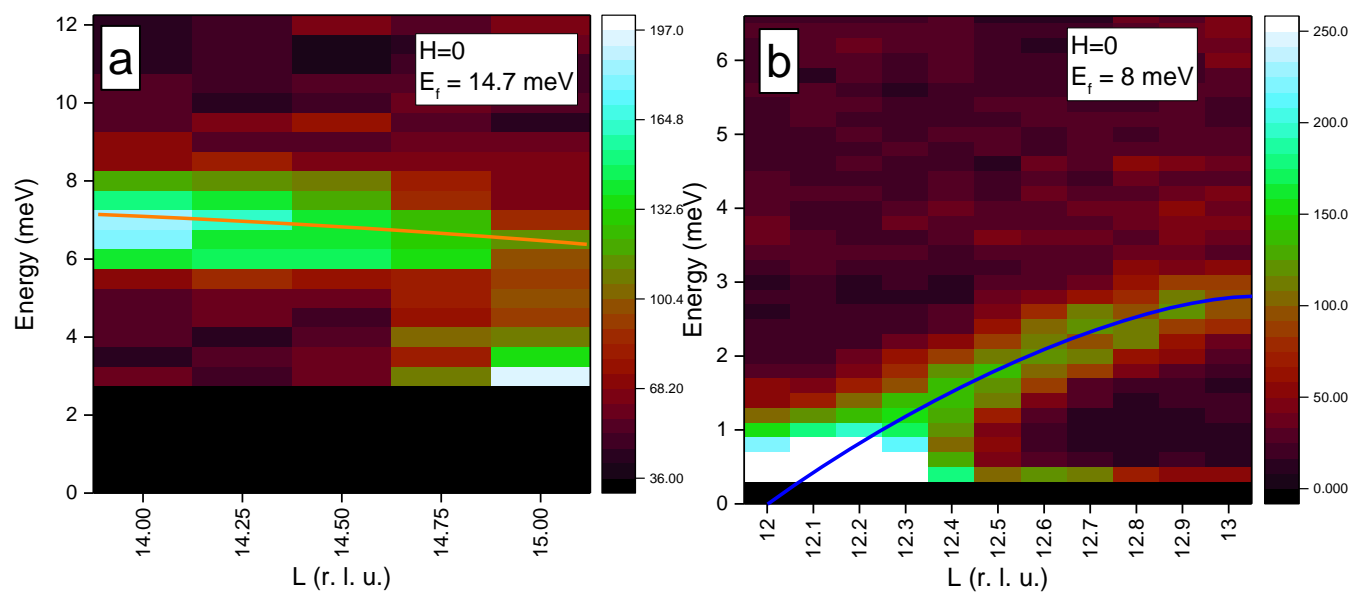

S4: Momentum-energy cut along L near (0, 0, 14) at a final neutron energy of 8 meV and  $T = 2$  K (a). Momentum-energy cut along L for (0, 0, 12) at a final neutron energy of 14.7 meV and  $T = 10$  K (b).
